# Supplementary material for: ClusterComm: Discrete Communication in Decentralized MARL using Internal Representation Clustering
Source: arXiv:2401.03504 source file (2024-01-07)
Supplement: Supplementary file 1 [file X_appendix.tex]

\section*{APPENDIX}
